# Supplementary material for: Ground Edge based LIDAR Localization without a Reflectivity Calibration for Autonomous Driving
Source: arXiv:1710.02192 source file (2017-10-05)
Supplement: Supplementary file 1 [file Appendix.tex]

\section{Appendix}
\label{Sec:Appendix}

 Assuming a column-wise vectorization of a 2D signal of size $ N_y \times N_x $, the first order forward difference discrete gradient is defined point-wise as
\begin{equation} \label{Gradient}
[\gXbf ]_n = 
\begin{pmatrix} 
[\gxXbf]_n \\ 
[\gyXbf]_n 
\end{pmatrix} = 
\begin{pmatrix}
[\Xbf]_{n + N_y} - [\Xbf]_n \\
[\Xbf]_{n+1} - [\Xbf]_n
\end{pmatrix}.	
\end{equation} 
were $ \g_x $ and $ \g_y $ represent the horizontal and vertical components, respectively. 
In a similar way, the discrete Laplacian operator $ \L : \mathbb{R}^N \rightarrow \mathbb{R}^N$ is defined point-wise as
\begin{equation} \label{Laplacian}
[\L \Xbf ]_n = -4 [\Xbf]_n + [\Xbf]_{n+1} + [\Xbf]_{n-1} + [\Xbf]_{n+N_y} + [\Xbf]_{n-N_y}	
\end{equation}

\subsection{Soft-tresholding algorithm}

\begin{algorithm}[t]
	\caption{ Anisotropic FISTA for gradient denoising.} \label{gradientFieldDenoising}
	\begin{algorithmic}[1]
		\BState \textbf{input:} Gradient $ \gYbf $, step $\gamma$, and thresholding const. $\tau$.
		
		\BState \textbf{for each component field $ k \in \{x,y\}$}
		\State \quad \textbf{set: }  $t \leftarrow 1$, $s^0 \leftarrow \g_k \Ybf $ 
		\BState \quad \textbf{repeat} %$T = T_{init}$ \mbox{through}  $T = T_{final}$
		\State \quad \quad $\pmb{s}^t \leftarrow \eta_{\tau}(\pmb{s}^{t-1} - \gamma \nabla \Dcal_3( \pmb{s}^{t-1}) ) $
		\State \quad \quad $ q_t \leftarrow \frac{1}{2} \left ( 1 + \sqrt{1+4 q^2_{t-1}} \right )$ 
		\State \quad \quad $\g_k \Xbf^t \leftarrow \pmb{s}^t + ( (q_{t-1} -1)/q^t) ( \pmb{s}^t - \pmb{s}^{t-1}) $.
		\State \quad \quad $ t \leftarrow t + 1$
		\BState \quad \textbf{until: } stopping criterion
		\State \textbf{return: } Denoised gradient of map-perspective $ \gXbf^t $
	\end{algorithmic}
\end{algorithm}
To denoise a map-perspective, we propose to apply the soft-thresholding \cite{Donoho95} to its gradient-field. This method solves the sparse promoting least squares optimization  
\begin{equation} \label{denoising}
	\g_k \Xbf = \arg \min\limits_{ \g_k \Xbf \in \Xcal_{\g} } 
	\left \{  
	\Dcal_3( \g_k \Xbf ) + \lambda \Rcal( \g_k \Xbf )
	\right \},
\end{equation}
for each horizontal and vertical $ k = \{x,y\}$ direction, independently. Here,
$\lambda > 0$ controls the amount of regularization (i.e., sparsity).
The first term in \eqref{denoising} measures the gradient fidelity defined in the least squares sense as
\begin{equation} \label{Eq:l2Fidelity}
	\Dcal_3( \g_k \Xbf ) =  \frac{1}{2} 
	\left \| \g_k \Ybf - \g_k \Xbf \right \|_{\ell_2}^2 
\end{equation}
while the second term is the non-smooth $\ell_1$ sparse promoting regularizer defined by
\begin{equation} \label{Eq:l1Regularizer}
	\Rcal( \g_k \Xbf ) = \| \g_k \Xbf \|_{\ell_1}.
\end{equation}
The optimization in \eqref{denoising} can be iteratively solved using the accelerated gradient descent in \cite{Nesterov1983} along with the non-convex proximity projection method of \cite{Beck.Teboulle2009b}. The complete Algorithm in \ref{gradientFieldDenoising} has a rate of convergence of $O(1/k^2)$.
